# Supplementary material for: Accelerating HEP simulations with Neural Importance Sampling
Source: arXiv:2401.09069 source file (2024-02-23)
Supplement: Supplementary file 1 [file forward_backward.tex]

In \cref{sec:training}, we described the forward-backward sampling approach to training normalizing flows for importance sampling in \cref{alg:trainingForwardBackward}, which we reproduce below for reference

\begin{algorithm}[H]
    % \SetAlgoLined
    \KwData{Parametric mapping $x=T(z,\theta)$ with associated PDF $p(x,\theta)$}
    \KwResult{Trained PDF $p(x,\theta)$}
     \For{M steps}{
        Set $\theta_0 \leftarrow \theta$\;
        Sample a batch $z_1,\dots,z_{n_\text{batch}}$ uniformly\;
        Compute the mapped batch $x_i = T(z_i,\theta_0)$ and their PDF values $p(x_i,\theta_0)$\; \label{algline:flow1}
        Compute function values $f(x_i)$\;
        Start tracking gradients with respect to $\theta$\;
     \For{N steps}{
        Compute the PDF values from the parametric PDF $p(x_i,\theta)$\; \label{algline:flow2}
        Estimate the loss $\hat{L} = \displaystyle \frac{1}{N} \sum_{i=1}^{n_\text{batch}} \frac{f(x_i)^2}{p(x_i,\theta)p(x_i,\theta_0)}$\;
        Compute $\nabla_\theta \hat{L}$ using backpropagation\;
        Set $\theta \leftarrow \theta - \eta \nabla_\theta \hat{L} $\;
        Reset gradients\;
     }
     }
     \Return $p(x,\theta)$\;
     {
     
     \caption{Forward-backward sampling training in \zunis }
     }
     \addtocounter{algocf}{-1}
    \end{algorithm}

As we discussed, this algorithm involves using the flow mapping twice: once on \cref{algline:flow1} in the forward direction for sampling and once on \cref{algline:flow2} in the backward direction for evaluating the PDF value of the sampled points. Because of the design of normalizing flows, computing the Jacobian of the mapping as it is being performed is very efficient and we could indeed obtain the PDF value of the sampled points during the forward mapping. This leads however to an incorrect evaluation of gradients. Indeed, let us consider the integral form of the loss function gradient
\begin{equation}
    \label{eq:goodgradient}
    \nabla_\theta \mathcal{L}(\theta) = \int dx f(x)^2 \nabla_\theta \frac{1}{p(x,\theta)}.
\end{equation}
Even when building an estimator for the gradient as proposed in \cref{eq:NISLossEstimator} \citep{mller2018neural}, sampling and evaluating the PDF value need to be separated. Indeed, evaluating the PDF during the forward pass corresponds to re-interpreting \cref{eq:badgradient} as
\begin{equation}
    \label{eq:badgradient}
    \nabla_\theta \mathcal{L}(\theta) \underset{?}{=} \int dy \left|\frac{dT}{dy} \right| f(T(y,\theta))^2 \nabla_\theta \frac{1}{\left|\frac{dT}{dy} \right|}.
\end{equation}
As far as the value of the PDF is concerned, we have indeed the following relation if $x = T(y,\theta)$
\begin{align}
    p(x,\theta) = \frac{\partial }{\partial \theta} \left|\frac{dT^{-1}(x,\theta)}{dx}\right|^{-1}= 
    p\left(T(y,\theta),\theta\right) = \left|\frac{dT}{dy}\right|(y,\theta).
\end{align}
However, depending on whether we keep $x$ or $y$ fix, the gradient with respect to $\theta$ takes different values:
\begin{align}
    \nabla_\theta p(x,\theta) = \frac{\partial }{\partial \theta} \left|\frac{dT^{-1}(x,\theta)}{dx}\right|^{-1} & = \frac{\partial p(x,\theta)}{\partial \theta}  \\
    \nabla_\theta p\left(T(y,\theta),\theta\right) = \frac{\partial }{\partial \theta} \left|\frac{dT(y,\theta)}{dy}\right| & = \frac{\partial \left(T(y,\theta),\theta\right)}{\partial \theta} + \frac{\partial p\left(T(y,\theta),\theta\right)}{\partial x} \frac{\partial T(y,\theta)}{d\theta}
\end{align}
so that we can conclude that
\begin{equation}
    \nabla_\theta p(x,\theta) \neq \nabla_\theta \left|\frac{dT(y,\theta)}{dy}\right|, 
\end{equation}
which means that we cannot use \cref{eq:badgradient} as a basis for our gradient loss estimator. If we want to truly estimate \cref{eq:goodgradient}, we need to sample $x$, consider it fixed, and then only compute its PDF value in a differentiable way, as done in \cref{alg:trainingForwardBackward}.

%%% Local Variables:
%%% mode: latex
%%% TeX-master: "../main"
%%% End:
