# Supplementary material for: Accelerating HEP simulations with Neural Importance Sampling
Source: arXiv:2401.09069 source file (2024-02-23)
Supplement: Supplementary file 2 [file nf_details.tex]

A coupling cell maps an input vector $\mathbf{x}=(x_1,\dots, x_n)$ to an output vector $\mathbf{y}=(y_1,\dots, y_n)$. This is done by separating the coordinate indices coordinate indices into two disjoint subsets $A$ and $B$ and applying the following transformation 
\begin{equation}
    \label{eq:CouplingCell}
    y = T(x):\; \left\{
    \begin{split}
       \mathbf{y}^A&=\mathbf{x}^A\\
        y^{b_1}&=C(\mathbf{x}^{b_1},m_{b_1}(\mathbf{x}^A))\\
        \vdots &\\
        y^{|B|}&=C(\mathbf{x}^{|B|}, m_{|B|}(\mathbf{x}^A)).
    \end{split}
    \right.
    \end{equation}
Because the coordinates in $A$ are not transformed, a choice of $(A,B)$ is called a mask.
Of course, because only some coordinates are transformed, we cannot hope to obtain a fully general probability distribution function approximator using a single coupling transform. While unproven, it seems however to suffice in practice to chain multiple cells with sufficiently shuffled masks.

A major advantage of coupling transforms is their low-cost Jacobian determinant evaluation. 
Indeed, from \cref{eq:CouplingCell}, one can readily derive the Jacobian matrix of the mapping $y = T(x)$:
\begin{equation}
    \label{eq:CouplingCellJacobian}
    \arraycolsep=1em
    J_T = 
    \det \left(
        \begin{array}{c|c}
        \bigsymbol{$\mathbbm{1}$} & \bigsymbol{0} \\ \hline
        \bigsymbol{$\circledast$ } & 
        {
            \arraycolsep=.3em
            \begin{matrix}
            c_{b_1} &  & 0\\
             & \ddots & \\
             0& & c_{b_{|B|}} 
            \end{matrix}
        } 
    \end{array}\right)  = \prod_{i=1}^{|B|} c_{b_i}.
\end{equation}
where $\circledast$ is a block matrix which contains hard-to-evaluate derivatives of $m_{b_i}$ but is irrelevant for computing the Jacobian determinant and 
\begin{equation}
    c_{b_i} = \frac{\partial C\left(x_{b_i}, m_{b_i}(x^A)\right)}{\partial{x_{b_i}}}.
\end{equation}
The Jacobian of coupling cells can therefore be computed analytically without resorting to backpropagation and expensive determintant computations.

Popular choices of the one-dimensional mappings $C$ include affine functions~\citep{dinh2014nice}, which are bijections $\mathbb{R}\mapsto \mathbb{R}$, piecewise polynomial functions~\citep{dinh2016density,mller2018neural} or piecewise spline~\citep{durkan2019neural} functions which can define bijections between finite intervals.
For each family of one-dimensional mapping, there are parameters that define the exact shape of the bijection, and it is through these parameters that non-trivial multivariate correlations are introduced: they are predicted by the neural networks $m_{b_i}(x^A)$ which only take the masked coordinates $x^A$ as inputs.

%%% Local Variables:
%%% mode: latex
%%% TeX-master: "../main"
%%% End:
