# Supplementary material for: Accelerating HEP simulations with Neural Importance Sampling
Source: arXiv:2401.09069 source file (2024-02-23)
Supplement: Supplementary file 3 [file phase_space_sampling.tex]

\zunis samples into the hypercube, whereas a phase space integral is an integral over $\mathbb{R}^{3n-4}$, with $n$ the number of final state particles, which can be written like
\begin{equation}
  \diff\phi_n(\{p_1,m_1\},\dots,\{p_n,m_n\}|Q)=\delta \left(\sum_{i=1}^n p_n-Q\right)\Pi_{i=1}^n \diff^4 p_i \delta(p_i^2-m_i^2)\theta(p_i^0-m_i)
\end{equation}
where the total momentum is $Q$ and the $p_i$ are the final state 4-vectors of particles with mass $m_i$. It is necessary to map the hypercube into the phase space in such a way that the kinematic conservation laws are respected (like momentum conservation), but at the same time the phase space should be covered evenly, in order to not induce as less additional variance as possible.  

This can be done by using the "RAMBO on diet" algorithm \cite{pltzer2013rambo}. The starting point is the decomposition of the multiparticle phase space with final states $\{p_i,m_i\}$ into subsequent $1\rightarrow 2$ decays with intermediate states $\{Q_i,M_i\}$ 
\begin{equation}
\begin{split}
    \diff\phi_n(\{p_1,m_1\},\dots,\{p_n,m_n\}|Q)&=
    \left(\prod_{i=2}^n \diff \phi_2 (\{p_{i-1},m_{i-1}\},\{Q_i, M_i\}|Q_{i-1})\right)\\\cdot&
    \left(\prod_{i=2}^n \theta(M_{i-1}-m_{i-1}-M_i) \theta\left(M_i-\sum_{k=i}^n m_k\right)\diff M_i^2\right)
    \label{equ:phin}
\end{split}
\end{equation}
with $Q_1=Q$ and $\{Q_n,M_n\}=\{p_n,m_n\}$ and without prefactors. Now, each of the two particle phase spaces can be expressed in the rest frame of its mother particle:
\begin{equation}
    \diff\phi_2(\{p_{i-1},m_{i-1}\},\{Q_i, M_i\}|Q_{i-1})=\rho (M_{i-1},M_i,m_{i-1})\diff\cos\theta_{i-1}\diff\phi_{i-1}.
\end{equation}
Here, $\rho$ is a weight that comes from the requirement of being on-shell:
\begin{equation}
\begin{split}
    &\mathbf{p}_{i-1}= -\mathbf{Q_i}= 4M_{i-1}\rho (M_{i-1},M_i,m_{i-1})(\cos\phi_{i-1}\sin\theta_{i-1}, \sin\phi_{i-1}\sin\theta_{i-1},\cos\theta_{i-1})^T \\
    & \rho=\frac{1}{8M_{i-1}^2}\sqrt{\left(M_{i-1}^2-(M_i-m_{i-1})^2\right)+\left(M_{i-1}^2-(M_i+m_{i-1})^2\right)}
\end{split}
\end{equation}
The zero-component can be then deduced from the on-shellness condition. The resulting final-state momenta can be brought into the centre-of-mass frame by a Lorentz boost, which preserves flatness. The flatness of the phase space generation is, when the angles are sampled in such a way that isotropy is guaranteed, only dependent on the sampling of the intermediate masses. This can be achieved by sampling them proportional to the measure of the two body phase spaces:
\begin{equation}
\begin{split}
     &\diff M_n(M_2,\dots,M_{n-1}|M_1;m_1,\dots,m_n)=\\&\rho(M_{n-1},m_n,m_{n-1})\\&\cdot\left(\prod_{i=2}^n \rho (M_{i-1},M_i,m_{i-1})\theta(M_{i-1}-m_{i-1}-M_i) \theta\left(M_i-\sum_{k=i}^n m_k\right)\diff M_i^2\right)
 \end{split}
 \label{equ:M}
\end{equation}
where $M_1$ is the mass of the initial state.

In the case of massless final states, this can be written as
\begin{equation}
    \diff M_n(M_2, \dots, M_{n-1}|M_1;0,\dots,0)=\frac{1}{8^{n-1}}\prod_{i=1}^{n-1}\frac{M^2_{i-1}-M_i^2}{M^2_{i-1}}\theta(M_{i-1}^2-M_i^2)\theta(M_i^2)\diff M_i^2
\end{equation}
It is always possible to write $M_i=u_2\dots u_i M_{1}$. The $u_i$ can be seen as the ratios of centre-of-mass energy being carried forward to the next decay at each step. Thus one gets
\begin{equation}
    \diff M_n(M_2, \dots, M_{n-1}|M_1;0,\dots,0)=\frac{1}{8^{n-1}}M_1^{2n-4}\prod_{i=1}^{n-1} u_i^{n-1-i}(1-u_i)\theta(1-u_i)\theta(u_i)\diff u_i
    \label{eq:ra}
\end{equation}
Using $v_i=(n+1-i)u^{n-i}_i-(n-i)u_i^{n+1-i}$, this can be expressed as
\begin{equation}
\begin{split}
    \diff M_n(M_2, \dots, M_{n-1}|M_1;0,\dots,0)&=\\ &=\frac{1}{8^{n-1}}M_1^{2n-4}\frac{1}{(n-1)!(n-2)!}\prod_{i=1}^{n-1} \theta(1-v_i)\theta(v_i)\diff v_i
\end{split}
\end{equation}
Starting from this description, it is possible to define an algorithm which performs a mapping from $[0,1]^{3n-4}$ into the flat massless $n$-particle phase space, which is the desired result. 
\begin{algorithm}[H]
\SetAlgoLined
\KwData{random numbers $r_0, \dots, r_{3n-4}, Q_1=E_{cm}, M_1=E_{cm}, M_n=0$}
\KwResult{Flat sampled momenta $\{p_1,\dots,p_n\}$ with weight $V_n$}
 
 \For{$i=2,\dots, n-1$}{
  solve $r_{i-1}=v_i=(n+1-i)u^{n-i}_i-(n-i)u_i^{n+1-i}$ for $u_i$\;
  $M_{i}\leftarrow u_2\dots u_i M_1$\;
  $\cos \theta_i \leftarrow 2r_{n-5+2i}-1, \phi_i\leftarrow 2\pi r_{n-4+2i}$\;
  $q_{i-1} \leftarrow 4 M_{i-1}\rho(M_{i-1},M_i,0)$\;
  $\sin\theta_{i-1}\leftarrow \sqrt{1-\cos \theta_{i-1}}$\;
  $\mathbf{p}_{i-1}= 4M_{i-1}\rho (M_{i-1},M_i,m_{i-1})(\cos\phi_{i-1}\sin\theta_{i-1}, \sin\phi_{i-1}\sin\theta_{i-1},\cos\theta_{i-1})^T $\;
  $p_{i-1}\leftarrow(q_{i-1},\mathbf{p}_{i-1})$,$Q_i\leftarrow (\sqrt{q_{i-1}^2+M_i^2},-\mathbf{p}_i)$\;
  boost $p_i$ and $Q_i$ by $\mathbf{Q}_{i-1}/Q_{i-1}^0$\;
 }
 $p_n\leftarrow Q_n$\;
 \caption{RAMBO on diet in the massless case}
\end{algorithm}
This algorithm can be further generalised to the massive case, for which it is only approximately flat.

In the example at hand, the phase space sampling was performed using the package  The package is also implemented in \textsc{PyTorch}, so that the phase space sampling can directly take the GPU-vectors sampled by \zunis and convert them into phase space points without a significant loss of performance.

%%% Local Variables:
%%% mode: latex
%%% TeX-master: "../main"
%%% End:
