# Supplementary material for: Accelerating HEP simulations with Neural Importance Sampling
Source: arXiv:2401.09069 source file (2024-02-23)
Supplement: Supplementary file 4 [file backward_sampling.tex]

\begin{algorithm}[H]
    \SetAlgoLined
    \KwData{Parametric PDF $p(x,\theta)$}
    \KwResult{Trained PDF $p(x,\theta)$}
     \For{M steps}{
        Sample a batch $x_1,\dots,x_{n_\text{batch}}$ from $q$\;
        Compute the sampling PDF values $q(x_i)$\;
        Compute function values $f(x_i)$\;
        Start tracking gradients with respect to $\theta$\;
     \For{N steps}{
        Compute the PDF values from the parametric PDF $p(x_i,\theta)$\;
        Estimate the loss $\hat{L} = \displaystyle \frac{1}{N} \sum_{i=1}^{n_\text{batch}} \frac{f(x_i)^2}{p(x,\theta)q(x)}$\;
        Compute $\nabla_\theta \hat{L}$ using backpropagation\;
        Set $\theta \leftarrow \theta - \eta \nabla_\theta \hat{L} $\;
        Reset gradients\;
     }
     }
     \Return $p(x,\theta)$\;
     \caption{Backward sampling training in \zunis}
     \label{alg:training}
    \end{algorithm}

%%% Local Variables:
%%% mode: latex
%%% TeX-master: "../main"
%%% End:
